# Supplementary material for: Fluorographene with Impurities as a Biomimetic Light-Harvesting Medium
Source: arXiv:1801.08509 ancillary file (2018-02-07)
Supplement: Supplementary file 1 [file Supporting_Informations.pdf]

# Fluorographene with Impurities as a Biomimetic Light-Harvesting Medium: Supporting Information

*Vladislav Sláma, Sayeh Rajabi and Tomáš Mančal*

Faculty of Mathematics and Physics, Charles University, Ke Karlovu 5, 121 16 Prague 2, Czech Republic

## 1 Fluorographene Lattice Parameters

Structure of pure fluorographene (FG) lattice was obtained from quantum chemistry calculation with periodic boundary conditions performed by Gaussian09 quantum chemistry package [1] with BLYP DFT functional and LANL2DZ basis [2]. Structure parameters are shown in Tab. 1 and Fig. 1. Lattice parameters for excitation transfer simulations were taken from projection of optimized FG structure into a plane.

## 2 Energetic Stability of the Impurities

Stability of the impurities in FG was investigated on three types of structures where fluorine vacancies were created in pairs. First type are sparse impurities where fluorine vacancies are far enough from each other to exhibit no mutual interaction (see Fig. 2a). Energies of these structures were calculated from energy difference between pure FG cluster and structure with two dissociated fluorine atoms forming double bond (db) $E_{8db} = E_{FG} - 8(E_{FG} - E_{1bd})$ . The second type are random impurities where fluorine vacancies were randomly created on the FG surface (Fig. 2b and 2c). The third type are compact impurities (moleculoids) where fluorine vacancies were created only on neighboring carbons resulting in $\pi$-conjugated graphene-like isles on FG surface (Fig. 2d). Stability of the impurities was compared using the same FG sheet and same number of fluorine vacancies (16 fluorines = 8 double bonds formed on FG surface) ($C_{150}F_{164}$) on 15 structures (1 sparse impurities, 13 random impurities, 1 compact impurity). Zero energy level was shifted to energy of a cluster with sparse impurities and compactness ("surface") of the defect was measured as a number of bonds between the defect and FG atoms. Geometries of all generated structures were optimized using DFT approach with BLYP functional with LANL2DZ double zeta valence basis in Gaussian09 quantum chemistry software. Comparison of ground state energies of optimized structure reveled that compact impurities are more stable and energetically favorable over more disordered impurities (Fig. 3).

## 3 Geometry Optimization

For geometry optimization we have compared DFT functionals (BLYP, B3LYP, BP86, CAM-B3LYP, $\omega$B97XD) and CI methods (CIS and CISD) with basis sets 6-31G(p,d) and LANL2DZ with the results of CISD/6-31G(p,d) geometry optimization. For comparison we used root-mean-square deviation

(RMSD) defined as $RMSD = \sqrt{\sum_i \frac{|r_i - r_i^{ref}|^2}{n}}$, where $r_i^{ref}$ are reference atomic coordinates obtained from CISD/6-31G(p,d) geometry optimization, and $r_i$ are atomic coordinates of the structure optimized by tested method.

## 4 Molecular Orbitals

For compact impurities (moleculoids) few highest occupied molecular orbitals ( $\pi$-molecular orbitals) are energetically higher than delocalized FG "molecular" orbitals (sigma-molecular orbitals). These pi-molecular orbitals are well localized on moleculoid with only small leakage into FG environment, and they are very similar to those from isolated impurity-like molecule (without FG).

## 5 Excited State Calculation

Results of excited state calculations depend on both structure of the molecule and the method used for the calculation. Correspondingly, two step procedure was used to compare the calculation methods. First, the structures were optimized by one of the two DFT functionals (BLYP and CAM-B3LYP) with LANL2DZ basis set. CAM-B3LYP DFT functional was chosen as the method providing the best geometries in the above geometry optimization comparison. BLYP was chosen because it is a very simple and fast method, and it was successfully used previously to obtain ground state properties of pure periodic fluorographene [2]. For calculation of the excited state properties TDDFT approach with B3LYP, BLYP, BP86, CAM-B3LYP, $\omega$B97, $\omega$B97XD functionals together with both 6-31G(p,d) and LANL2DZ basis sets and ZIndo/S were used. In the comparison we focused on transition energies of the two lowest excited states $^1L_a$ (mainly HOMO→LUMO transition) and $^1L_b$ (mainly HOMO-1→LUMO and HOMO→LUMO+1 transition). Our main aim is to obtain the same systematic error for all different molecule sizes and shapes in order to describe wide range of molecules with the same accuracy. The performance of different methods is shown in Tabs. 3-6. Coefficients $a$ and $b$ are parameters of linear regression between experimental and calculated excitation energies and $r^2$ is the coefficient of determination. The most suitable combination of methods was determined as BLYP/LANL2DZ for geometry optimization and $\omega$B97XD/LANL2DZ for excited state properties (Fig. 9). Other methods usually perform well for one excited state, but the other is described less accurately (e.g. CAM-B3LYP/LANL2DZ on Fig. 9).

## 6 Fluorographene/Vacuum Excited State Properties Comparison

Comparison of excited state properties for two perylene and anthanthrene geometries (optimal geometry and FG geometry) and perylene-like and anthanthrene-like impurities on FG surface is shown in Tab. 7. The optimal geometry corresponds to optimized structure of the isolated molecule in vacuum without the FG. The FG geometry corresponds to geometry optimized with FG where only hydrogens were added after the optimization to replace missing bonds between defect and the FG. The positions of hydrogens were then optimized keeping all carbons frozen at FG geometry. Excited state properties and transition dipoles were calculated for both geometries in vacuum. From this comparison it can be seen that change of the geometry of isolated molecule from vacuum optimal geometry to geometry in fluorographene results only in very small change of transition dipole moment (~1%) and slightly higher change of transition energy of $S_1$ transition. Whereas changing the environment of the impurity (molecule) from vacuum to FG environment (without changing the geometry) produce dramatic charge of transition dipole moment (enhancement of transition dipole in compare to the vacuum) and lowers

transition energy of $S_1$ transition. Change of the environment from vacuum to the FG does not change the symmetry of the transition density. Highest occupied and lowest unoccupied molecular orbitals as well as transition density are localized in the area of the impurity with only small leakage into FG environment (see figures in the main text).

# 7 Comparison of Redfield/Förster Calculations with Exact Propagation of Density Matrix

Large aggregates, for which HEOM computations are not feasible, follow essentially the same principles as the small ones e studied in the main tex. They could be studied to a large degree of confidence with Redfield and Förster theories. To demonstrate this idea, we compare the exact results of HEOM with Redfield and Förster theories in their corresponding parameter regimes. We employ implementation of Redfield and Förster theories from the Quantarhei software package [3] to perform the computations for both perturbative theories. We take three perylene moleculoids with relatively small resonance couplings: 3.2, 7.8 and 11.3 cm$^{-1}$. We assume that the initial population is localized on one of the sites and find the density matrix in the site basis representation. With reorganization energy $\lambda = 15$ cm$^{-1}$, one expects the Förster theory to describe the population transfer among the three monomers correctly. The result is compared with HEOM and excellent agreement between the two is found (see Fig. 10a ). In the regime of large $J_{ij}/\lambda$, one needs to apply the Redfield theory. We consider another aggregate within which resonance couplings are ten times bigger than previous example (32, 78, 113 cm$^{-1}$) and check secular Redfield theory against HEOM for the same reorganization energy. Once again the two computations demonstrate very similar population transfer dynamics as can be seen in Fig. 10b. In the regime where couplings and reorganization energy are comparable, non-secular Redfield theory still shows good agreement to the exact computations of HEOM. As an example, we also consider $\lambda = 50$ cm$^{-1}$ in Fig. 10c , where resonance couplings are set as before: 32, 78, 113 cm$^{-1}$. Even here, where Redfield theory is outside its strict regime of validity, it still yields rather accurate results at both short and long times. These examples clearly show that the two effective theories can explain the energy transfer between the selected moleculoids very well. Such an agreement paves the way towards studying larger aggregates.

## Tables

| parameter | value |
|---|---|
| C-C bond length | 1.5945Å |
| C-F bond length | 1.4443Å |
| C-C-C angle | 111.71° |
| C-C-F angle | 107.138° |
| C-C-C-C dihedral angle | 54.06° |

Tab. 1: Structure parameters for the fluorographene sheet.

| | B3LYP 6-31G(d,p) | B3LYP LANL2DZ | BLYP 6-31G(d,p) | BLYP LANL2DZ | BP86 6-31G(d,p) | BP86 LANL2DZ | CAM-B3LYP 6-31G(d,p) | CAM-B3LYP LANL2DZ |
|---|---|---|---|---|---|---|---|---|
| Triphenylene | 5.33E-03 | 8.93E-03 | 9.78E-03 | 1.39E-02 | 8.75E-03 | 1.24E-02 | 3.19E-03 | 6.40E-03 |
| Pyrene | 5.44E-03 | 9.15E-03 | 9.84E-03 | 1.40E-02 | 9.03E-03 | 1.28E-02 | 3.28E-03 | 6.69E-03 |
| Picene | 6.15E-03 | 1.01E-02 | 1.13E-02 | 1.57E-02 | 9.85E-03 | 1.39E-02 | 3.52E-03 | 7.08E-03 |
| Phenanthrene | 5.33E-03 | 9.12E-03 | 9.84E-03 | 1.42E-02 | 8.93E-03 | 1.28E-02 | 3.17E-03 | 6.58E-03 |
| Perylene | 5.32E-03 | 8.89E-03 | 9.75E-03 | 1.39E-02 | 8.73E-03 | 1.24E-02 | 3.20E-03 | 6.38E-03 |
| Dibenz[a,j]anthracene | 5.81E-03 | 9.81E-03 | 1.07E-02 | 1.53E-02 | 9.37E-03 | 1.35E-02 | 3.36E-03 | 6.89E-03 |
| Dibenz[a,h]anthracene | 6.08E-03 | 1.02E-02 | 1.12E-02 | 1.59E-02 | 9.83E-03 | 1.40E-02 | 3.48E-03 | 7.16E-03 |
| Dibenz[a,c]anthracene | 5.70E-03 | 9.57E-03 | 1.04E-02 | 1.47E-02 | 9.18E-03 | 1.31E-02 | 3.37E-03 | 6.87E-03 |
| Coronene | 5.64E-03 | 9.20E-03 | 1.01E-02 | 1.42E-02 | 9.13E-03 | 1.27E-02 | 3.46E-03 | 6.68E-03 |
| Chrysene | 5.77E-03 | 9.65E-03 | 1.06E-02 | 1.50E-02 | 9.42E-03 | 1.34E-02 | 3.36E-03 | 6.85E-03 |
| Bisanthrene | 5.60E-03 | 9.17E-03 | 1.01E-02 | 1.41E-02 | 9.00E-03 | 1.26E-02 | 3.38E-03 | 6.60E-03 |
| Benzo[e]pyrene | 5.42E-03 | 9.00E-03 | 9.86E-03 | 1.40E-02 | 8.86E-03 | 1.25E-02 | 3.26E-03 | 6.47E-03 |
| Benzo[b]chrysene | 6.26E-03 | 1.05E-02 | 1.14E-02 | 1.62E-02 | 1.00E-02 | 1.44E-02 | 3.60E-03 | 7.43E-03 |
| Benzo[a]pyrene | 5.82E-03 | 9.66E-03 | 1.05E-02 | 1.49E-02 | 9.48E-03 | 1.34E-02 | 3.46E-03 | 6.96E-03 |
| Benz[a]anthracene | 5.75E-03 | 9.87E-03 | 1.06E-02 | 1.52E-02 | 9.42E-03 | 1.36E-02 | 3.39E-03 | 7.09E-03 |
| Anthanthrene | 5.83E-03 | 9.64E-03 | 1.04E-02 | 1.48E-02 | 9.46E-03 | 1.33E-02 | 3.50E-03 | 6.98E-03 |

| | CIS 6-31G(d,p) | CIS LANL2DZ | CISD LANL2DZ | wB97 6-31G(d,p) | wB97 LANL2DZ | wB97XD 6-31G(d,p) | wB97XD LANL2DZ |
|---|---|---|---|---|---|---|---|
| Triphenylene | 0.6287 | 0.6299 | 7.23E-03 | 4.99E-03 | 7.32E-03 | 3.77E-03 | 6.89E-03 |
| Pyrene | 4.72E-03 | 6.90E-03 | 7.62E-03 | 5.08E-03 | 7.57E-03 | 3.81E-03 | 7.03E-03 |
| Picene | 5.85E-03 | 8.27E-03 | 7.77E-03 | 5.43E-03 | 8.01E-03 | 4.15E-03 | 7.65E-03 |
| Phenanthrene | 5.60E-03 | 7.87E-03 | 8.00E-03 | 4.93E-03 | 7.42E-03 | 3.73E-03 | 6.99E-03 |
| Perylene | 4.20E-03 | 5.28E-03 | 7.03E-03 | 5.07E-03 | 7.37E-03 | 3.75E-03 | 6.83E-03 |
| Dibenz[a,j]anthracene | 3.66E-03 | 6.11E-03 | 7.54E-03 | 5.20E-03 | 7.78E-03 | 3.92E-03 | 7.35E-03 |
| Dibenz[a,h]anthracene | 4.83E-03 | 7.25E-03 | 7.87E-03 | 5.26E-03 | 7.97E-03 | 4.04E-03 | 7.64E-03 |
| Dibenz[a,c]anthracene | 3.73E-03 | 6.03E-03 | 7.45E-03 | 5.26E-03 | 7.86E-03 | 3.94E-03 | 7.32E-03 |
| Coronene | 2.93E-03 | 5.10E-03 | 6.77E-03 | 5.31E-03 | 7.65E-03 | 3.94E-03 | 7.03E-03 |
| Chrysene | 6.29E-03 | 8.58E-03 | 7.85E-03 | 5.16E-03 | 7.71E-03 | 3.96E-03 | 7.33E-03 |
| Bisanthrene | 3.26E-03 | 4.89E-03 | 6.59E-03 | 5.26E-03 | 7.64E-03 | 3.86E-03 | 7.00E-03 |
| Benzo[e]pyrene | 3.57E-03 | 5.59E-03 | 7.02E-03 | 5.08E-03 | 7.40E-03 | 3.82E-03 | 6.91E-03 |
| Benzo[b]chrysene | 5.43E-03 | 7.99E-03 | 8.12E-03 | 5.45E-03 | 8.29E-03 | 4.19E-03 | 7.91E-03 |
| Benzo[a]pyrene | 5.00E-03 | 7.22E-03 | 7.58E-03 | 5.26E-03 | 7.86E-03 | 3.99E-03 | 7.36E-03 |
| Benz[a]anthracene | 4.64E-03 | 7.07E-03 | 8.13E-03 | 5.22E-03 | 7.96E-03 | 3.96E-03 | 7.52E-03 |
| Anthanthrene | 4.14E-03 | 6.35E-03 | 7.31E-03 | 5.36E-03 | 7.93E-03 | 3.98E-03 | 7.32E-03 |

Tab. 2: RMSD in Angstroms for the structure of aromatic hydrocarbons optimized by different methods compared to CISD/6-31G(p,d) optimization.

| molname | exp[eV] | B3LYP 6-31G(d,p) | B3LYP LANL2DZ | BLYP 6-31G(d,p) | BLYP LANL2DZ | BP86 6-31G(d,p) | BP86 LANL2DZ |
|---|---|---|---|---|---|---|---|
| Bisanthrene | 1.87 | 1.7142 | 1.7262 | 1.5389 | 1.5486 | 1.5414 | 1.5613 |
| Perylene | 2.85 | 2.777 | 2.7886 | 2.5291 | 2.5386 | 2.5379 | 2.5614 |
| Anthanthrene | 2.86 | 2.727 | 2.772 | 2.4721 | 2.5112 | 2.4824 | 2.5315 |
| Benzo[a]pyrene | 3.22 | 3.0567 | 3.1123 | 2.7644 | 2.8103 | 2.7762 | 2.8347 |
| Benzo[b]chrysene | 3.4 | 3.0128 | 3.0802 | 2.6274 | 2.6844 | 2.6378 | 2.7074 |
| Benz[a]anthracene | 3.63 | 3.269 | 3.3273 | 2.918 | 2.9659 | 2.9298 | 2.9935 |
| Pyrene | 3.71 | 3.5763 | 3.6286 | 3.2908 | 3.3337 | 3.3077 | 3.364 |
| Coronene | 3.72 | 3.3245 | 3.3916 | 3.0004 | 3.0531 | 3.0189 | 3.0845 |
| Benzo[e]pyrene | 3.73 | 3.6202 | 3.67 | 3.2795 | 3.3206 | 3.2968 | 3.3524 |
| Picene | 3.8 | 3.5944 | 3.6659 | 3.1705 | 3.226 | 3.1871 | 3.256 |
| Dibenz[a,c]anthracene | 3.84 | 3.3774 | 3.4377 | 2.9966 | 3.0464 | 3.0095 | 3.0755 |
| Dibenz[a,j]anthracene | 3.84 | 3.3858 | 3.4421 | 2.9938 | 3.0409 | 3.0069 | 3.0707 |
| Dibenz[a,h]anthracene | 3.86 | 3.2921 | 3.438 | 2.9915 | 3.0433 | 2.9276 | 3.0722 |
| Chrysene | 3.89 | 3.64 | 3.7634 | 3.2718 | 3.321 | 3.2881 | 3.3524 |
| Phenanthrene | 4.24 | 4.114 | 4.1779 | 3.7752 | 3.8248 | 3.7967 | 3.8645 |
| Triphenylene | 4.54 | 3.8533 | 3.8925 | 3.4989 | 3.5329 | 3.5177 | 3.5663 |
| a | | 0.8464 | 0.8727 | 0.7686 | 0.7834 | 0.7713 | 0.7926 |
| b | | 0.2555 | 0.2232 | 0.2068 | 0.1967 | 0.2061 | 0.1918 |
| r^2 | | 0.9185 | 0.9247 | 0.8944 | 0.8991 | 0.8855 | 0.8993 |

| molname | exp[eV] | CAM-B3LYP 6-31G(d,p) | CAM-B3LYP LANL2DZ | wB97 6-31G(d,p) | wB97 LANL2DZ | wB97XD 6-31G(d,p) | wB97XD LANL2DZ | Zindo |
|---|---|---|---|---|---|---|---|---|
| Bisanthrene | 1.87 | 1.9443 | 1.958 | 2.1249 | 2.1595 | 1.9724 | 2.0028 | 1.9535 |
| Perylene | 2.85 | 3.0879 | 3.1007 | 3.3311 | 3.3749 | 3.1146 | 3.1498 | 2.8642 |
| Anthanthrene | 2.86 | 3.0166 | 3.0693 | 3.2352 | 3.3191 | 3.0317 | 3.0994 | 2.7059 |
| Benzo[a]pyrene | 3.22 | 3.3848 | 3.4515 | 3.6168 | 3.7187 | 3.4084 | 3.4928 | 3.0098 |
| Benzo[b]chrysene | 3.4 | 3.4396 | 3.5185 | 3.7107 | 3.8271 | 3.485 | 3.5838 | 3.1411 |
| Benz[a]anthracene | 3.63 | 3.6652 | 3.731 | 3.9161 | 4.0637 | 3.7003 | 3.7877 | 3.3449 |
| Pyrene | 3.71 | 3.8811 | 3.945 | 4.0977 | 4.2058 | 3.8926 | 3.9758 | 3.3789 |
| Coronene | 3.72 | 3.3545 | 3.7534 | 3.8726 | 3.5569 | 3.7011 | 3.4274 | 2.8853 |
| Benzo[e]pyrene | 3.73 | 3.9818 | 4.0425 | 4.2095 | 4.3186 | 4.0108 | 4.0932 | 3.4715 |
| Picene | 3.8 | 4.0044 | 4.0926 | 4.2399 | 4.3764 | 4.0403 | 4.1484 | 3.4682 |
| Dibenz[a,c]anthracene | 3.84 | 3.8035 | 3.8757 | 4.0666 | 4.1873 | 3.8489 | 3.9455 | 3.419 |
| Dibenz[a,j]anthracene | 3.84 | 3.8112 | 3.8763 | 4.0736 | 4.1847 | 3.8547 | 3.9451 | 3.4516 |
| Dibenz[a,h]anthracene | 3.86 | 3.7913 | 3.8676 | 4.0526 | 4.1757 | 3.8349 | 3.9337 | 3.3819 |
| Chrysene | 3.89 | 4.0799 | 4.1659 | 4.3136 | 4.449 | 4.1098 | 4.2171 | 3.5472 |
| Phenanthrene | 4.24 | 4.4485 | 4.5265 | 4.6542 | 4.7857 | 4.4703 | 4.5734 | 3.8498 |
| Triphenylene | 4.54 | 4.1826 | 4.496 | 4.3916 | 4.7441 | 4.1987 | 4.251 | 3.5763 |
| a | | 0.8998 | 0.9762 | 0.9188 | 0.9871 | 0.9095 | 0.9236 | 0.6723 |
| b | | 0.4116 | 0.2393 | 0.5958 | 0.4489 | 0.4269 | 0.4365 | 0.8204 |
| r^2 | | 0.9069 | 0.9641 | 0.9358 | 0.9153 | 0.9380 | 0.8983 | 0.8693 |

Tab. 3: Transition energies of $^1L_a$ state for geometry optimized at BLYP/LANL2DZ level.

| molname | exp[eV] | B3LYP 6-31G(d,p) | B3LYP LANL2DZ | BLYP 6-31G(d,p) | BLYP LANL2DZ | BP86 6-31G(d,p) | BP86 LANL2DZ |
|---|---|---|---|---|---|---|---|
| Bisanthrene | 1.87 | 1.8365 | 1.853 | 1.6417 | 1.6566 | 1.6437 | 1.6697 |
| Perylene | 2.85 | 2.9144 | 2.9301 | 2.6481 | 2.6618 | 2.6565 | 2.6855 |
| Anthanthrene | 2.86 | 2.8681 | 2.9189 | 2.5951 | 2.6394 | 2.6048 | 2.6601 |
| Benzo[a]pyrene | 3.22 | 3.2045 | 3.2669 | 2.8935 | 2.9457 | 2.9048 | 2.9707 |
| Benzo[b]chrysene | 3.4 | 3.1568 | 3.2319 | 2.7572 | 2.8211 | 2.767 | 2.8446 |
| Benz[a]anthracene | 3.63 | 3.4096 | 3.475 | 3.046 | 3.1001 | 3.0572 | 3.1283 |
| Pyrene | 3.71 | 3.727 | 3.7854 | 3.4285 | 3.4756 | 3.4439 | 3.5066 |
| Coronene | 3.72 | 3.2462 | 3.293 | 2.944 | 2.9837 | 2.9593 | 3.0101 |
| Benzo[e]pyrene | 3.73 | 3.7691 | 3.825 | 3.4162 | 3.4623 | 3.4331 | 3.4949 |
| Picene | 3.8 | 3.7623 | 3.8414 | 3.3235 | 3.3854 | 3.3395 | 3.416 |
| Dibenz[a,c]anthracene | 3.84 | 3.5255 | 3.5926 | 3.1322 | 3.188 | 3.1445 | 3.2179 |
| Dibenz[a,j]anthracene | 3.84 | 3.5209 | 3.5838 | 3.1191 | 3.1715 | 3.1316 | 3.2023 |
| Dibenz[a,h]anthracene | 3.86 | 3.439 | 3.5999 | 3.0483 | 3.191 | 3.0597 | 3.2207 |
| Chrysene | 3.89 | 3.794 | 3.9291 | 3.4134 | 3.4684 | 3.4293 | 3.5004 |
| Phenanthrene | 4.24 | 4.2687 | 4.3398 | 3.9206 | 3.9762 | 3.9419 | 4.0169 |
| Triphenylene | 4.54 | 4.2242 | 4.2985 | 3.828 | 3.8793 | 3.8491 | 3.9218 |
| a | | 0.8881 | 0.9201 | 0.8066 | 0.8275 | 0.8136 | 0.8381 |
| b | | 0.2528 | 0.2073 | 0.1986 | 0.1775 | 0.1871 | 0.1685 |
| r^2 | | 0.9183 | 0.9269 | 0.8891 | 0.9036 | 0.8890 | 0.9040 |

| molname | exp[eV] | CAM-B3LYP 6-31G(d,p) | CAM-B3LYP LANL2DZ | wB97 6-31G(d,p) | wB97 LANL2DZ | wB97XD 6-31G(d,p) | wB97XD LANL2DZ | Zindo |
|---|---|---|---|---|---|---|---|---|
| Bisanthrene | 1.87 | 2.0961 | 2.1143 | 2.3054 | 2.3457 | 2.1267 | 2.1634 | 2.0928 |
| Perylene | 2.85 | 3.2466 | 3.2638 | 3.5071 | 3.5575 | 3.2732 | 3.3147 | 3.0057 |
| Anthanthrene | 2.86 | 3.1818 | 3.2407 | 3.4208 | 3.5126 | 3.1986 | 3.2739 | 2.8462 |
| Benzo[a]pyrene | 3.22 | 3.5542 | 3.6283 | 3.8032 | 3.9139 | 3.5783 | 3.6715 | 3.1531 |
| Benzo[b]chrysene | 3.4 | 3.597 | 3.6847 | 3.8802 | 4.0082 | 3.6409 | 3.7499 | 3.2754 |
| Benz[a]anthracene | 3.63 | 3.8187 | 3.8925 | 4.0852 | 4.2414 | 3.8527 | 3.9502 | 3.4764 |
| Pyrene | 3.71 | 4.048 | 4.1187 | 4.2772 | 4.3947 | 4.0597 | 4.1511 | 3.5155 |
| Coronene | 3.72 | 3.8276 | 3.575 | 4.0474 | 3.7591 | 3.8615 | 3.607 | 3.0259 |
| Benzo[e]pyrene | 3.73 | 4.143 | 4.2107 | 4.3798 | 4.4986 | 4.1717 | 4.2626 | 3.6024 |
| Picene | 3.8 | 4.1817 | 4.2784 | 4.4232 | 4.5714 | 4.2164 | 4.3347 | 3.6151 |
| Dibenz[a,c]anthracene | 3.84 | 3.9632 | 4.0431 | 4.2358 | 4.3666 | 4.0078 | 4.1137 | 3.554 |
| Dibenz[a,j]anthracene | 3.84 | 3.9561 | 4.0288 | 4.2278 | 4.3489 | 3.9986 | 4.0985 | 3.5765 |
| Dibenz[a,h]anthracene | 3.86 | 3.9581 | 4.0424 | 4.2285 | 4.3622 | 4.0008 | 4.1093 | 3.5238 |
| Chrysene | 3.89 | 4.2498 | 4.3446 | 4.4918 | 4.6389 | 4.2786 | 4.396 | 3.6868 |
| Phenanthrene | 4.24 | 4.6114 | 4.6975 | 4.8236 | 4.9661 | 4.6328 | 4.7457 | 3.9847 |
| Triphenylene | 4.54 | 4.5767 | 4.6672 | 4.7751 | 4.9231 | 4.6084 | 4.7257 | 3.7101 |
| a | | 0.9497 | 0.9718 | 0.9484 | 0.9839 | 0.9524 | 0.9775 | 0.6697 |
| b | | 0.4300 | 0.4022 | 0.6782 | 0.6455 | 0.4512 | 0.4345 | 0.9671 |
| r^2 | | 0.9591 | 0.9301 | 0.9592 | 0.9162 | 0.9629 | 0.9310 | 0.8693 |

Tab. 4: Transition energies of $^1L_a$ state for geometry optimized at CAM-B3LYP/LANL2DZ level.

| molname | exp[eV] | B3LYP 6-31G(d,p) | B3LYP LANL2DZ | BLYP 6-31G(d,p) | BLYP LANL2DZ | BP86 6-31G(d,p) | BP86 LANL2DZ |
|---|---|---|---|---|---|---|---|
| Benzo[a]pyrene | 3.06 | 3.3147 | 3.3502 | 2.9942 | 3.0226 | 3.0093 | 3.051 |
| Dibenz[ah]anthracene | 3.14 | 4.012 | 3.3298 | 2.9156 | 2.9485 | 3.3936 | 2.976 |
| Benzanthracene | 3.22 | 3.4367 | 3.4744 | 3.0436 | 3.0786 | 3.0579 | 3.1074 |
| Benzo[b]chrysene | 3.23 | 3.3661 | 3.4086 | 2.9359 | 2.9717 | 2.9492 | 2.9989 |
| Picene | 3.3 | 3.4576 | 3.5024 | 3.0522 | 3.091 | 3.0666 | 3.1193 |
| Dibenz[a,c]anthracene | 3.31 | 3.4917 | 3.5319 | 3.0911 | 3.1266 | 3.106 | 3.1562 |
| Dibenz[a,j]anthracene | 3.32 | 3.2932 | 3.333 | 2.8999 | 2.9369 | 2.9131 | 2.9637 |
| Benzo[e]pyrene | 3.37 | 3.5196 | 3.5531 | 3.1453 | 3.1716 | 3.1613 | 3.2023 |
| Chrysene | 3.43 | 4.2629 | 3.6864 | 3.3379 | 3.3785 | 3.3551 | 3.4102 |
| Pyrene | 3.53 | 3.6385 | 3.6726 | 3.3739 | 3.4019 | 3.3928 | 3.4335 |
| Phenanthrene | 3.76 | 3.8665 | 3.8932 | 3.5218 | 3.5429 | 3.5399 | 3.5777 |
| Triphenylene | 3.89 | 4.0678 | 4.1343 | 3.6811 | 3.7283 | 3.7027 | 3.7685 |
| a | | 0.721 | 0.953 | 0.977 | 0.980 | 0.815 | 0.995 |
| b | | 1.207 | 0.352 | -0.135 | -0.113 | 0.465 | -0.131 |
| r^2 | | 0.289 | 0.911 | 0.871 | 0.873 | 0.627 | 0.873 |

| molname | exp[eV] | CAM-B3LYP 6-31G(d,p) | CAM-B3LYP LANL2DZ | wB97 6-31G(d,p) | wB97 LANL2DZ | wB97XD 6-31G(d,p) | wB97XD LANL2DZ | Zindo |
|---|---|---|---|---|---|---|---|---|
| Benzo[a]pyrene | 3.06 | 3.5861 | 3.6249 | 3.7309 | 3.7949 | 3.6008 | 3.6546 | 3.0869 |
| Dibenz[ah]anthracene | 3.14 | 3.6594 | 3.6968 | 3.865 | 3.9242 | 3.6871 | 3.7419 | 3.2049 |
| Benzanthracene | 3.22 | 3.7771 | 3.8186 | 4.9471 | 3.9883 | 3.8007 | 3.8604 | 3.2655 |
| Benzo[b]chrysene | 3.23 | 3.694 | 3.7381 | 3.8549 | 3.9234 | 3.7188 | 3.7777 | 3.1848 |
| Picene | 3.3 | 3.8015 | 3.8468 | 3.9869 | 4.0535 | 3.8235 | 3.8839 | 3.2774 |
| Dibenz[a,c]anthracene | 3.31 | 3.8598 | 3.8987 | 4.0577 | 4.1177 | 3.8895 | 3.9445 | 3.3383 |
| Dibenz[a,j]anthracene | 3.32 | 3.6629 | 3.7018 | 3.8694 | 3.9288 | 3.6907 | 3.7459 | 3.2003 |
| Benzo[e]pyrene | 3.37 | 3.834 | 3.8689 | 4.0072 | 4.0633 | 3.8491 | 3.8994 | 3.2839 |
| Chrysene | 3.43 | 3.9442 | 3.985 | 4.1121 | 4.1755 | 3.9579 | 4.0147 | 3.3851 |
| Pyrene | 3.53 | 3.8475 | 3.8825 | 3.9607 | 4.0187 | 3.8519 | 3.9018 | 3.2758 |
| Phenanthrene | 3.76 | 4.1505 | 4.1789 | 4.3131 | 4.367 | 4.1594 | 4.2063 | 3.5612 |
| Triphenylene | 3.89 | 4.4145 | 4.2184 | 4.6078 | 4.4475 | 4.4465 | 4.5535 | 3.7951 |
| a | | 0.8983 | 0.7059 | 0.6469 | 0.7165 | 0.8930 | 0.9259 | 0.7224 |
| b | | 0.8162 | 1.4858 | 1.9228 | 1.6452 | 0.8545 | 0.8024 | 0.8797 |
| r^2 | | 0.8910 | 0.8790 | 0.1998 | 0.8546 | 0.8780 | 0.8615 | 0.8587 |

Tab. 5: Transition energies of $^1L_b$ state for geometry optimized at BLYP/LANL2DZ level.

| | | B3LYP | B3LYP | BLYP | BLYP | BP86 | BP86 |
|---|---|---|---|---|---|---|---|
| molname | exp[eV] | 6-31G(d,p) | LANL2DZ | 6-31G(d,p) | LANL2DZ | 6-31G(d,p) | LANL2DZ |
| Benzo[a]pyrene | 3.06 | 3.4614 | 3.5031 | 3.127 | 3.1607 | 3.1417 | 3.1897 |
| Dibenz[a,h]anthracene | 3.14 | 4.1583 | 3.4827 | 3.5239 | 3.0865 | 3.5392 | 3.1146 |
| Benzanthracene | 3.22 | 3.5863 | 3.6302 | 3.1812 | 3.2215 | 3.1952 | 3.251 |
| Benzo[b]chrysene | 3.23 | 3.5199 | 3.569 | 3.0745 | 3.1151 | 3.0873 | 3.1429 |
| Picene | 3.3 | 3.6118 | 3.6633 | 3.1924 | 3.2369 | 3.2063 | 3.2659 |
| Dibenz[a,c]anthracene | 3.31 | 3.6396 | 3.6862 | 3.227 | 3.268 | 3.2415 | 3.2983 |
| Dibenz[a,j]anthracene | 3.32 | 3.4457 | 3.4916 | 3.0401 | 3.0825 | 3.0528 | 3.1099 |
| Benzo[e]pyrene | 3.37 | 3.6706 | 3.7094 | 3.2835 | 3.314 | 3.2991 | 3.3456 |
| Chrysene | 3.43 | 4.4032 | 3.847 | 3.4818 | 3.7709 | 3.4985 | 3.8094 |
| Pyrene | 3.53 | 3.7842 | 3.8242 | 3.5085 | 3.5415 | 3.5269 | 3.5736 |
| Phenanthrene | 3.76 | 4.017 | 4.049 | 3.6611 | 3.6866 | 3.6788 | 3.7223 |
| Triphenylene | 3.89 | 4.0126 | 4.058 | 3.6468 | 3.6862 | 3.6653 | 3.7204 |
| a | | 0.5610 | 0.7715 | 0.6718 | 0.8580 | 0.6781 | 0.8679 |
| b | | 1.8799 | 1.1019 | 1.0585 | 0.4474 | 1.0522 | 0.4452 |
| r^2 | | 0.2013 | 0.8848 | 0.5385 | 0.6773 | 0.5398 | 0.6750 |

| | | CAM-B3LYP | CAM-B3LYP | wB97 | wB97 | wB97XD | wB97XD | Zindo |
|---|---|---|---|---|---|---|---|---|
| molname | exp[eV] | 6-31G(d,p) | LANL2DZ | 6-31G(d,p) | LANL2DZ | 6-31G(d,p) | LANL2DZ | |
| Benzo[a]pyrene | 3.06 | 3.752 | 3.7978 | 3.9166 | 3.9894 | 3.767 | 3.8294 | 3.2238 |
| Dibenz[a,h]anthracene | 3.14 | 3.8236 | 3.8677 | 4.0455 | 4.1128 | 3.8508 | 3.9141 | 3.342 |
| Benzanthracene | 3.22 | 3.9407 | 3.9889 | 4.1364 | 4.172 | 3.9635 | 4.0312 | 3.4002 |
| Benzo[b]chrysene | 3.23 | 3.8629 | 3.9141 | 4.0393 | 4.1156 | 3.8869 | 3.9546 | 3.3227 |
| Picene | 3.3 | 3.9725 | 4.0252 | 4.1742 | 4.2494 | 3.9937 | 4.063 | 3.4185 |
| Dibenz[a,c]anthracene | 3.31 | 4.0211 | 4.0669 | 4.2312 | 4.2996 | 4.0504 | 4.114 | 3.4695 |
| Dibenz[a,j]anthracene | 3.32 | 3.8301 | 3.8757 | 4.0517 | 4.1191 | 3.857 | 3.9206 | 3.3384 |
| Benzo[e]pyrene | 3.37 | 3.9987 | 4.0396 | 4.1846 | 4.2481 | 4.0136 | 4.0715 | 3.4156 |
| Chrysene | 3.43 | 4.1135 | 4.1615 | 4.2966 | 4.3683 | 4.1265 | 4.192 | 3.5245 |
| Pyrene | 3.53 | 4.0089 | 4.0501 | 4.1376 | 4.2029 | 4.0136 | 4.0713 | 3.4066 |
| Phenanthrene | 3.76 | 4.314 | 4.3485 | 4.4891 | 4.5507 | 4.3222 | 4.3769 | 3.696 |
| Triphenylene | 3.89 | 4.3532 | 4.3953 | 4.5708 | 4.6342 | 4.3689 | 4.4289 | 3.9266 |
| a | | 0.719 | 0.707 | 0.713 | 0.709 | 0.701 | 0.690 | 0.716 |
| b | | 1.569 | 1.656 | 1.779 | 1.860 | 1.648 | 1.748 | 1.037 |
| r^2 | | 0.884 | 0.879 | 0.849 | 0.853 | 0.876 | 0.868 | 0.856 |

Tab. 6: Transition energies of $^1L_b$ state for geometry optimized at CAM-B3LYP/LANL2DZ level.

| name | $E_{0\to1}[eV]$ | $E_{0\to1}[cm^{-1}]$ | $\lvert\overrightarrow{d}_{0\to1}\rvert\ [AU]$ | $\lvert\overrightarrow{d}_{0\to1}\rvert\ [D]$ |
|---|---|---|---|---|
| Perylene (opt. geometry) | 3.1498 | 25405 | 2.4945 | 6.3404 |
| Perylene (FG geometry) | 3.0987 | 24993 | 2.4795 | 6.3023 |
| Perylene-like impurity on FG | 2.7715 | 22354 | 2.8753 | 7.3083 |
| Anthathrene (opt. geometry) | 3.0994 | 24999 | 2,5379 | 6.4507 |
| Anthathrene (FG geometry) | 2.9894 | 24111 | 2,5771 | 6.5503 |
| Anthathrene-like impurity on FG | 2.6948 | 21736 | 3.4617 | 8.7988 |

Tab. 7: Transition energies and transition dipole moments of perylene and anthanthrene molecules in vacuum optimized and fluorographene geometries, together with the same for perylene- and anthanthrene-like impurities in fluorographene.

## Figures

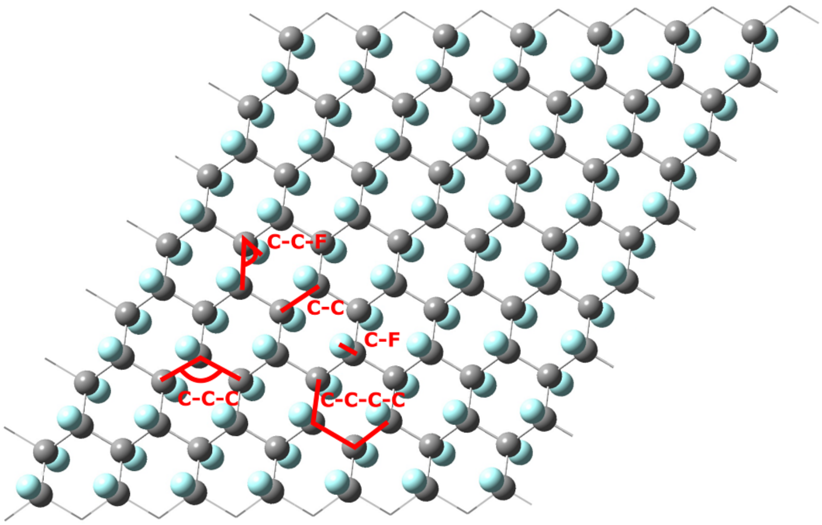


Fig. 1: Definition of the structure parameters for fluorographene sheet.

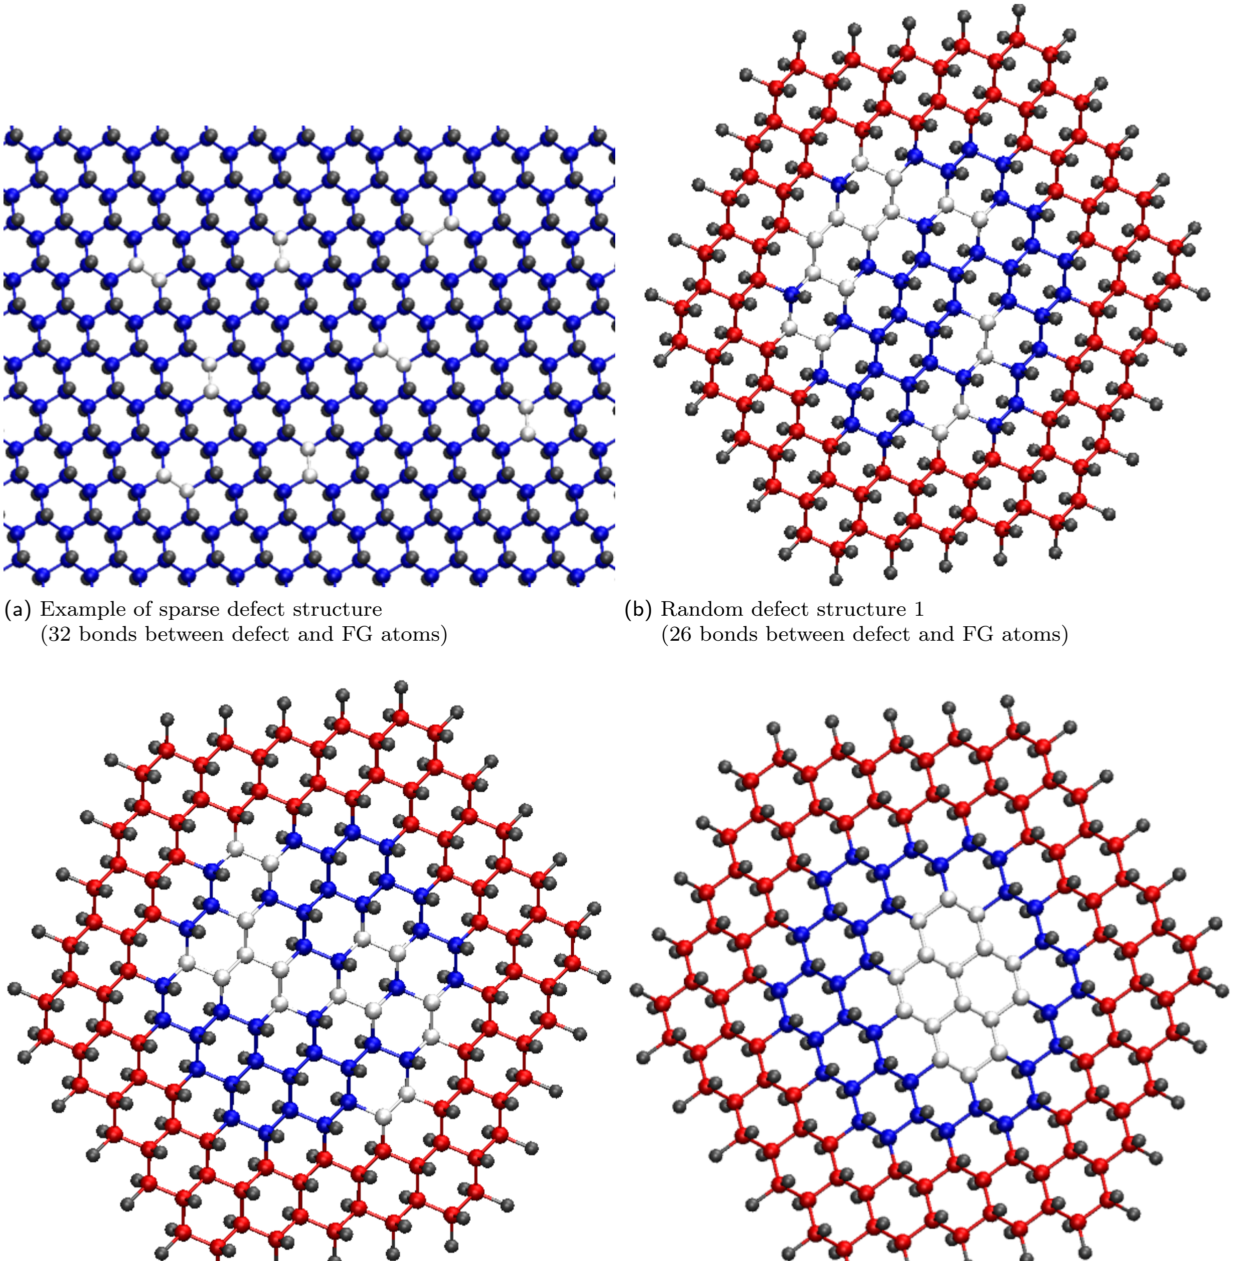

(a) Example of sparse defect structure
(32 bonds between defect and FG atoms)

(b) Random defect structure 1
(26 bonds between defect and FG atoms)

(c) Random defect structure 2
(28 bonds between defect and FG atoms)

(d) Compact defect structure
(10 bonds between defect and FG atoms)

Fig. 2: Examples of fluorographene cluster structures with 16 disconnected fluorine atoms (8 double bonds formed between fluorographene carbons). Gray color represents fluorine atoms, white represents carbon atoms belonging to the impurity, red represent border carbons of the fluorographene cluster – we do not allow formation of impurities on these atoms to minimize cluster border effects on impurity properties – and blue represents inner fluorographene carbons from which fluorine can be dissociated and impurity can be formed.

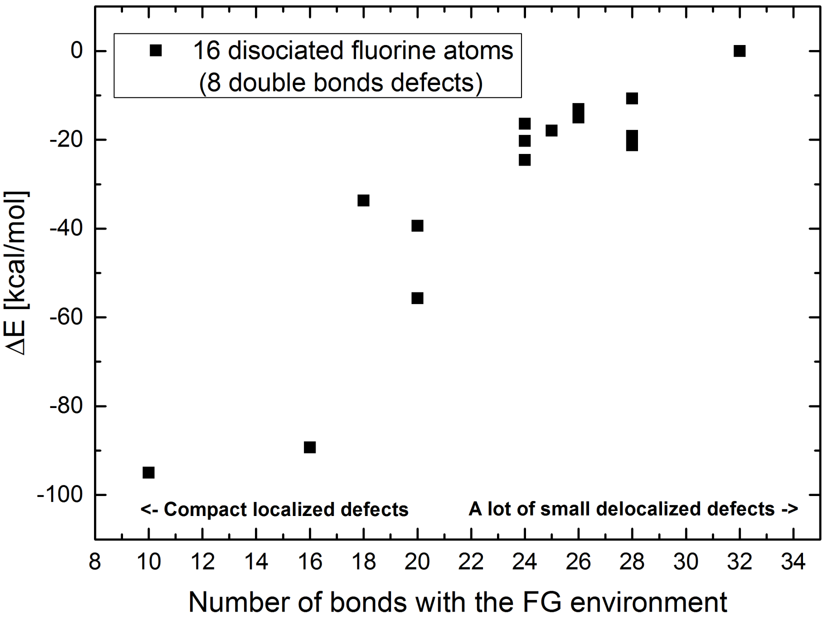


Fig. 3: Energetic stability of various defects for 16 dissociated fluorine atoms.

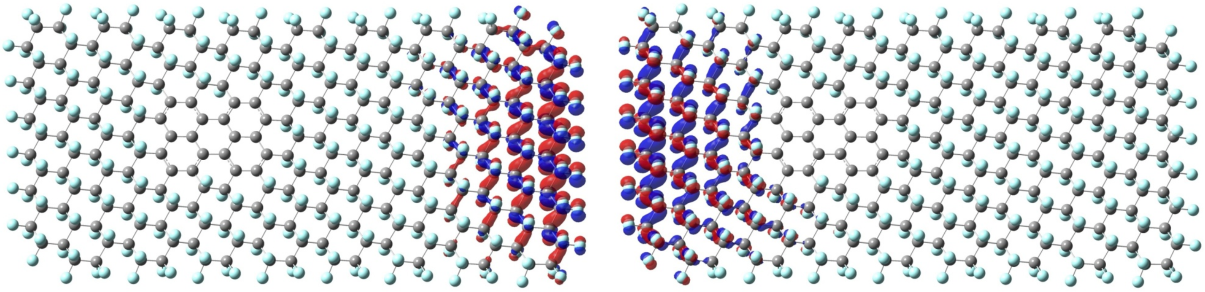

(a) FG with perylene moleculoid HOMO-6

(b) FG with perylene moleculoid HOMO-5

Fig. 4: Example of selocalized occupied molecular orbitals of fluorographene with perylene-like impurity.

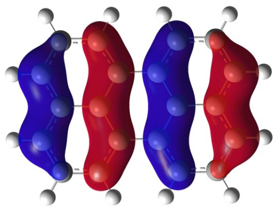

(a) Perylene HOMO-4

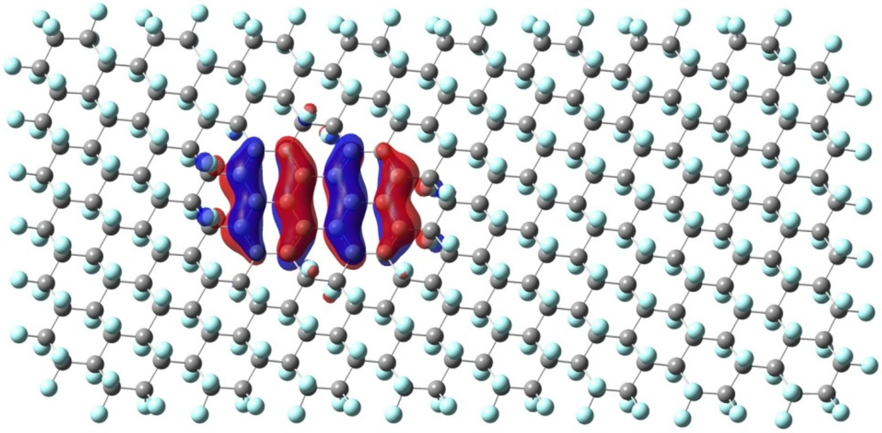

(b) FG with perylene moleculoid HOMO-4

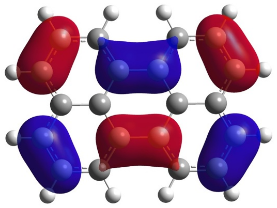

(c) Perylene HOMO-3

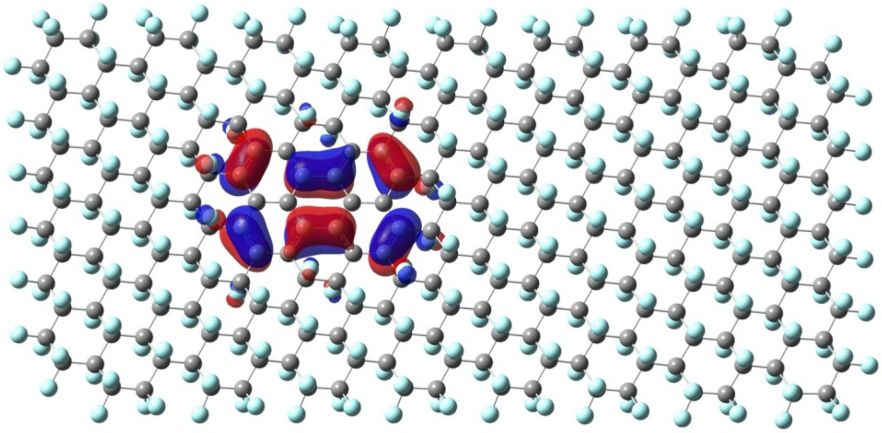

(d) FG with perylene moleculoid HOMO-3

Fig. 5: Localized occupied molecular orbitals of fluorographene with impurity and comparison with molecular orbital of isolated perylene molecule.

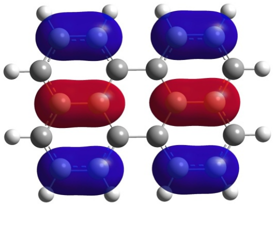

(a) Perylene HOMO-2

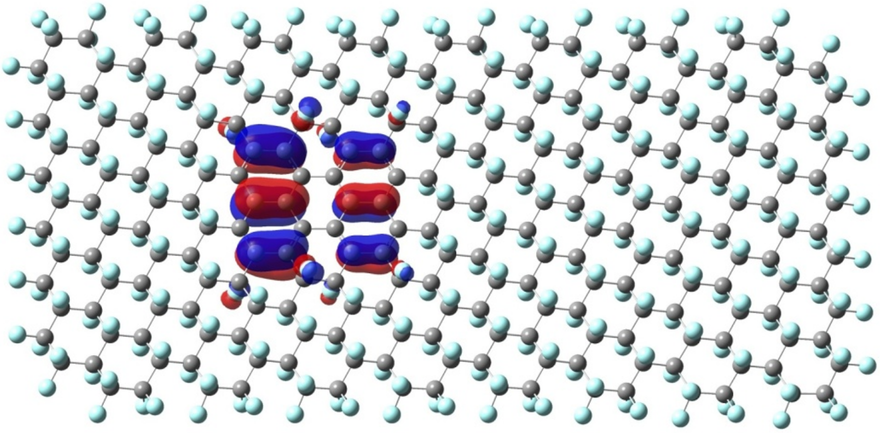

(b) FG with perylene moleculoid HOMO-2

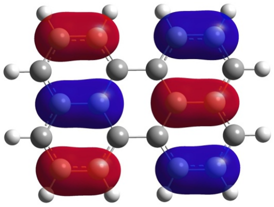

(c) Perylene HOMO-1

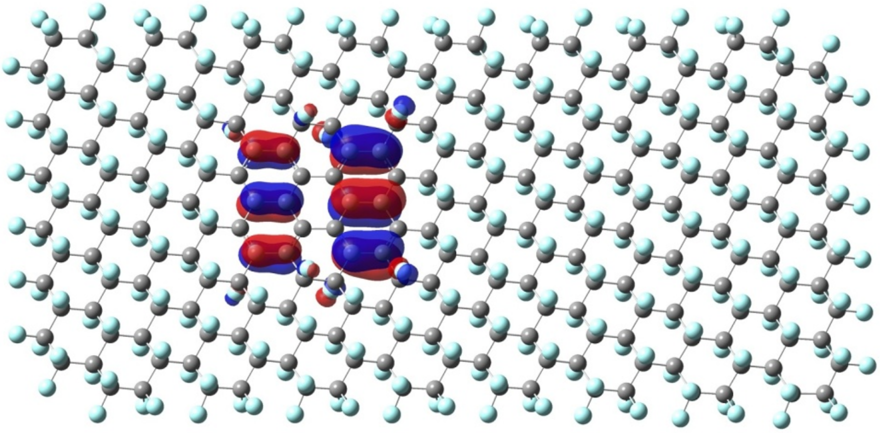

(d) FG with perylene moleculoid HOMO-1

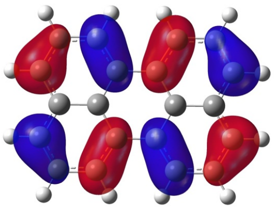

(e) Perylene HOMO

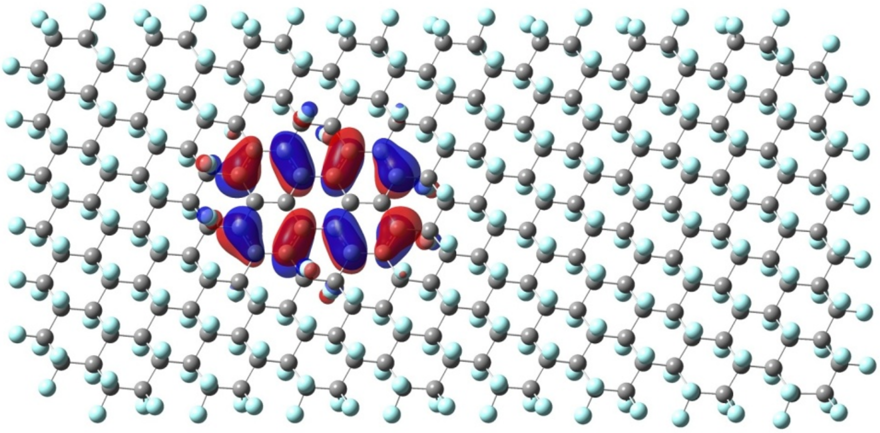

(f) FG with perylene moleculoid HOMO

Fig. 6: Localized occupied molecular orbitals of fluorographene with impurity and comparison with molecular orbital of isolated perylene molecule.

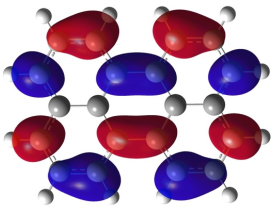

(a) Perylene LUMO

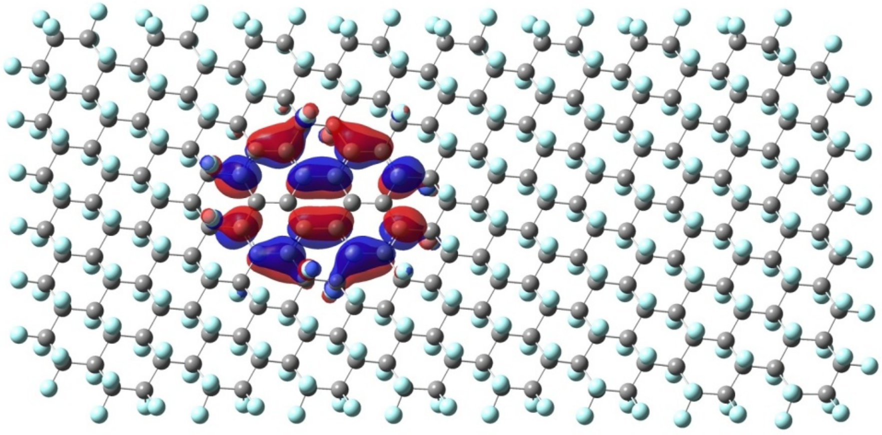

(b) FG with perylene moleculoid LUMO

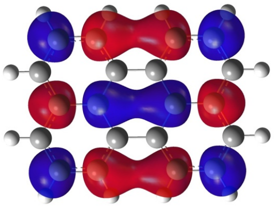

(c) Perylene LUMO+1

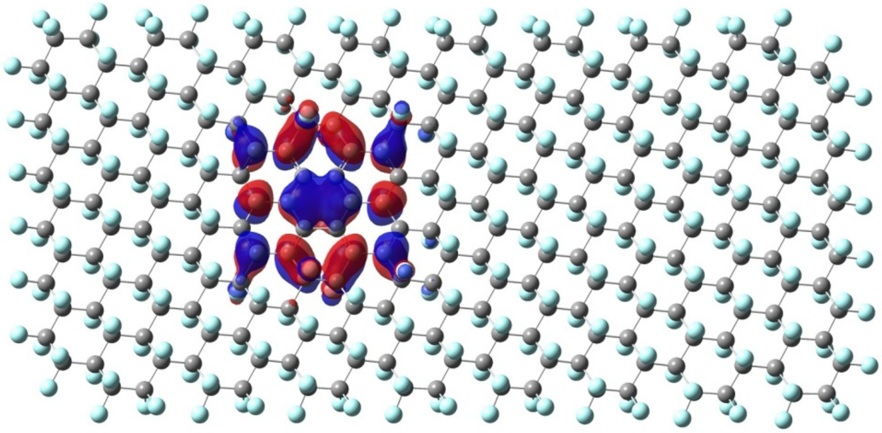

(d) FG with perylene moleculoid LUMO+1

Fig. 7: Localized unoccupied molecular orbitals of fluorographene with impurity and comparison with molecular orbital of isolated perylene molecule.

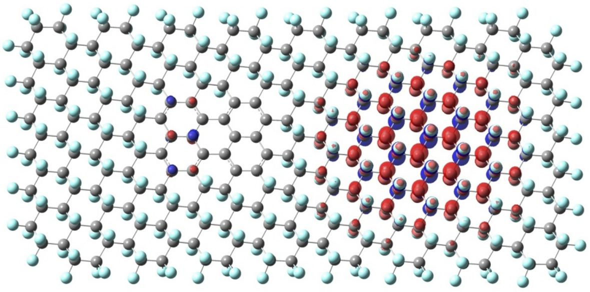

(a) FG with perylene moleculoid LUMO+2

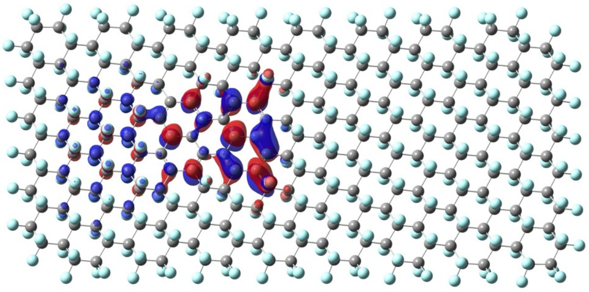

(b) FG with perylene moleculoid LUMO+3

Fig. 8: Delocalized unoccupied molecular orbitals of fluorographene with perylene-like impurity.

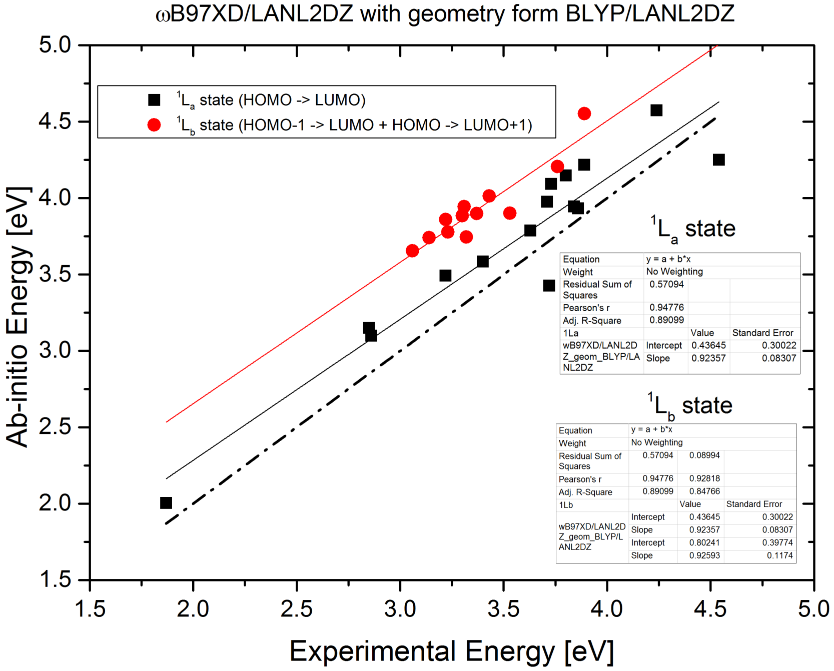


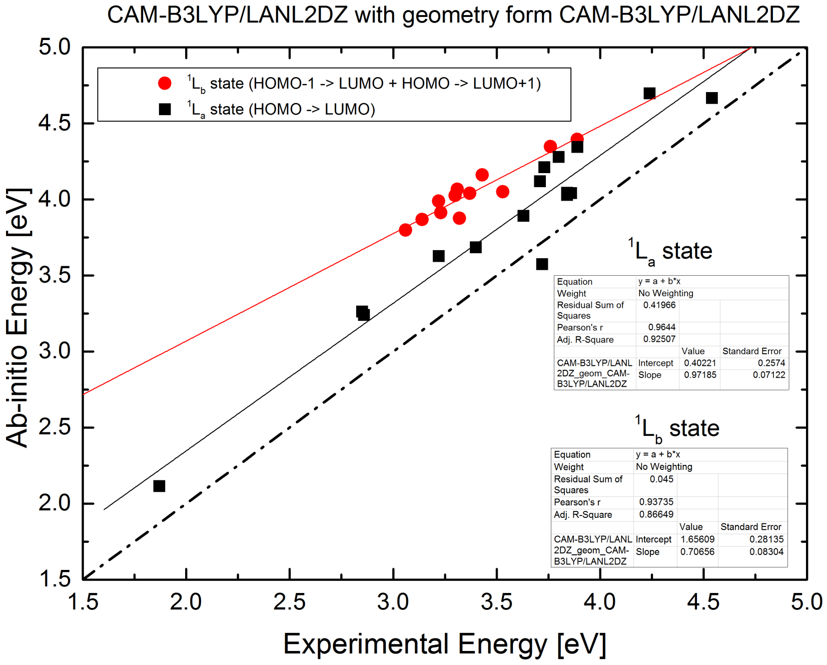


Fig. 9: Comparison ofdifferent methods for transition energy calculation.

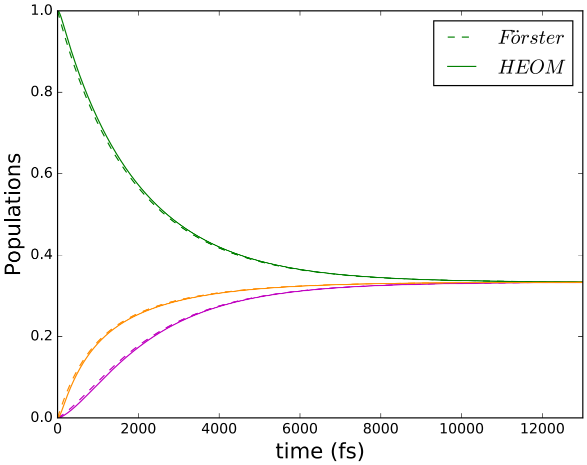


(a)

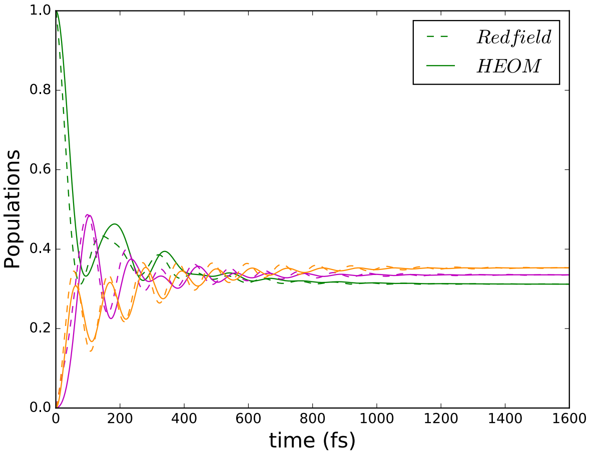


(b)

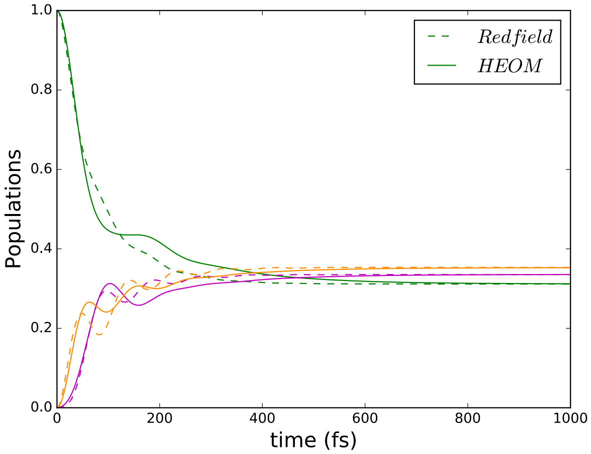


(c)

Fig. 10: Population dynamics for three perylene-like moleculoids with small (a) and large (b) resonance couplings compared to reorganization energy $\lambda = 15\ \mathrm{cm}^{-1}$. Förster and Redfield theories explain the energy transfer in the corresponding regimes of couplings very well. In (c) we take the same large resonance couplings together with $\lambda = 50\ \mathrm{cm}^{-1}$. Redfield theory is still a reliable approximation.

## References

[1] M. J. Frisch, G. W. Trucks, H. B. Schlegel, G. E. Scuseria, M. A. Robb, J. R. Cheeseman, G. Scalmani, V. Barone, G. A. Petersson, H. Nakatsuji, X. Li, M. Caricato, A. Marenich, J. Bloino, B. G. Janesko, R. Gomperts, B. Mennucci, H. P. Hratchian, J. V. Ortiz, A. F. Izmaylov, J. L. Sonnenberg, D. Williams-Young, F. Ding, F. Lipparini, F. Egidi, J. Goings, B. Peng, A. Petrone, T. Henderson, D. Ranasinghe, V. G. Zakrzewski, J. Gao, N. Rega, G. Zheng, W. Liang, M. Hada, M. Ehara, K. Toyota, R. Fukuda, J. Hasegawa, M. Ishida, T. Nakajima, Y. Honda, O. Kitao, H. Nakai, T. Vreven, K. Throssell, J. J. A. Montgomery, J. E. Peralta, F. Ogliaro, M. Bearpark, J. J. Heyd, E. Brothers, K. N. Kudin, V. N. Staroverov, T. Keith, R. Kobayashi, J. Normand, K. Raghavachari, A. Rendell, J. C. Burant, S. S. Iyengar, J. Tomasi, M. Cossi, J. M. Millam, M. Klene, C. Adamo, R. Cammi, J. W. Ochterski, R. L. Martin, K. Morokuma, O. Farkas, J. B. Foresman, , and D. J. Fox, Gaussian 09, Revision D.01, 2016.

[2] R. Zbořil, F. Karlickỳ, A. B. Bourlinos, T. A. Steriotis, A. K. Stubos, V. Georgakilas, K. Šafářová, D. Jančík, C. Trapalis, and M. Otyepka, small **6**, 2885 (2010).

[3] T. Mančal, Quantarhei: Open Quantum Systems Theory for Molecular Systems, 2017, [Online: http://www.github.com/tmancal74/quantarhei; accessed Jan 25, 2018].
